# Supplementary material for: Detecting topological invariants in chiral symmetric insulators via losses
Source: arXiv:1611.09670 ancillary file (2016-12-14)
Supplement: Supplementary file 1 [file supplemental_material.pdf]

# Supplemental Material to "Detecting topological invariants in chiral symmetric insulators via losses"

Tibor Rakovszky,[1] János K. Asbóth,[2] and Andrea Alberti[3]
[1] Max-Planck-Institut für Physik komplexer Systeme, Nöthnitzer Str. 38, 01187 Dresden, Germany
[2] Institute for Solid State Physics and Optics, Wigner Research Centre for Physics, Hungarian Academy of Sciences, H-1525 Budapest P.O. Box 49, Hungary
[3] Institut für Angewandte Physik, Universität Bonn, Wegelerstr. 8, D-53115 Bonn, Germany
(Dated: December 2016)

## I. SOLVING THE TIME EVOLUTION FOR A SINGLE INITIAL STATE

Here we derive the exact form of the time evolved conditional wavefunction $|\tilde{\Psi}(t)\rangle$, that we will use in the subsequent appendices to compute double averaged quantities.

As already noted in the main text, we can express the conditional wavefunction after the $j$-th driving cycle as

$$|\tilde{\Psi}(t=jT)\rangle = \sum_n \left[\alpha_n(j)|A\rangle_n + \beta_n(j)|B\rangle_n\right], \tag{1}$$

where we use the states

$$|A\rangle_n = \frac{|n\rangle + \hat{\Gamma}|n\rangle}{\sqrt{2}} \qquad |B\rangle_n = \frac{|n\rangle - \hat{\Gamma}|n\rangle}{\sqrt{2}}, \tag{2}$$

defined for each pair of quasienergy eigenstates $\{|n\rangle, \hat{\Gamma}|n\rangle\}$. The state $|A\rangle_n$ ($|B\rangle_n$) has support on sublattice $A$ ($B$). Solving the time evolution then simplifies to finding the coefficients $\alpha_n(j)$ and $\beta_n(j)$. These evolve in time according to

$$\begin{pmatrix}\alpha_n(j+1)\\ \beta_n(j+1)\end{pmatrix} = \underbrace{\begin{pmatrix}\cos\varepsilon_n & -i\sqrt{1-p_M}\sin\varepsilon_n\\ -i\sin\varepsilon_n & \sqrt{1-p_M}\cos\varepsilon_n\end{pmatrix}}_{D_n}\begin{pmatrix}\alpha_n(j)\\ \beta_n(j)\end{pmatrix}, \tag{3}$$

with initial conditions

$$\alpha_n(0) = \sqrt{2}\langle n|\Psi(0)\rangle \qquad \beta_n(0) = 0. \tag{4}$$

In order to solve Eq. (3), we will need the eigenvalues and right eigenvectors of the $2\times 2$ matrix $D_n$. These satisfy

$$D_n v_{n,\pm} = \lambda_{n,\pm} v_{n,\pm}. \tag{5}$$

The eigenvalues $\lambda_{n,\pm}$ obey the following relations

$$\lambda_{n,+}\lambda_{n,-} = \sqrt{1-p_M}; \tag{6a}$$

$$\lambda_{n,+} + \lambda_{n,-} = (1+\sqrt{1-p_M})\cos\varepsilon_n. \tag{6b}$$

One can then decompose the coefficients of the initial state as

$$\begin{pmatrix}\alpha_n(0)\\ \beta_n(0)\end{pmatrix} = \alpha_n(0)\begin{pmatrix}1\\ 0\end{pmatrix} = \alpha_n(0)\left(A_{n,+}v_{n,+} + A_{n,-}v_{n,-}\right) \tag{7}$$

The (unnormalized) eigenvectors $v_{n,\pm}$ and the corresponding amplitudes $A_{n,\pm}$ are

$$v_{n,\pm} = \begin{pmatrix}1\\ i\frac{\lambda_{n,\pm}-\cos\varepsilon_n}{\sqrt{1-p_M}\sin\varepsilon_n}\end{pmatrix} \qquad A_{n,\pm} = \frac{\cos\varepsilon_n - \lambda_{n,\mp}}{\lambda_{n,\pm}-\lambda_{n,\mp}}. \tag{8}$$

The solution to Eq. (3) then takes the form

$$\begin{pmatrix} \alpha_n(j) \\ \beta_n(j) \end{pmatrix} = \alpha_n(0)(A_{n,+}\lambda_{n,+}^j v_{n,+} + A_{n,-}\lambda_{n,-}^j v_{n,-}). \tag{9}$$

Using the formulas (6)-(9) and the initial condition (4) we can express $\beta_n(j)$ explicitly as

$$\beta_n(j) = -i\sqrt{2}\langle n|\Psi(0)\rangle \sin\varepsilon_n \frac{\lambda_{n,+}^j - \lambda_{n,-}^j}{\lambda_{n,+} - \lambda_{n,-}}. \tag{10}$$

This is the result valid for a specific starting state $|\Psi(0)\rangle$. The other set of coefficients, $\{\alpha_n(j)\}$, can be similarly determined, however they do not feature in any of the relevant quantities, since the measurement process only concerns the states on sublattice $B$.

## II. COMPUTATION OF $\langle\langle t\rangle\rangle$ AND $\langle\langle \Delta x\rangle\rangle$

Here we show how to arrive at the formulas for $\langle\langle \Delta x\rangle\rangle$ and $\langle\langle t\rangle\rangle$ presented in the main text. Using the definitions of the main text, for a particle, initially in the state $|x,a\rangle$, the probability of finding it in the state $|y,b\rangle$ after $j$ driving periods is given by

$$s_{(x,a)\to(y,b)}(j) = 2p_M\left|\sum_n \langle y,b|n\rangle \beta_n^{(x,a)}(j)\right|^2, \tag{11}$$

where we have used that $\langle y,b|B\rangle_n = \sqrt{2}\langle y,b|n\rangle$. Building on the results of the previous Supplemental Material, we have for each initial state

$$\beta_n^{(x,a)} = \sqrt{2}\langle n|x,a\rangle\Lambda_n(j) \qquad \Lambda_n(j) = -i\sin\varepsilon_n \frac{\lambda_{n,+}^j - \lambda_{n,-}^j}{\lambda_{n,+} - \lambda_{n,-}}, \tag{12}$$

where $\Lambda_n(j)$ denotes all the factors that depend on $j$, $\varepsilon_n$ or $p_M$. With this notation the double averaged displacement can be written as

$$\langle\langle \Delta x\rangle\rangle = \frac{4}{NL}\sum_{n,m}\sum_{y,b}(y-x)\langle y,b|n\rangle\langle m|y,b\rangle \sum_{x,a}\langle n|x,a\rangle\langle x,a|m\rangle \sum_j \Lambda_n(j)\Lambda_m(j)^*. \tag{13}$$

Note that due to the factor $(y-x)$ we have two terms: in the first term we can sum over $x$ while in the second term we can sum over $y$ by using the following two formulas:

$$\sum_x\sum_a \langle n|x,a\rangle\langle x,a|m\rangle = \langle n|\hat{P}_A|m\rangle = \frac{1}{2}\delta_{nm} \tag{14}$$

$$\sum_y\sum_b \langle y,b|n\rangle\langle m|y,b\rangle = \langle m|\hat{P}_B|n\rangle = \frac{1}{2}\delta_{nm}. \tag{15}$$

Thus in Eq. (13) we only need to keep the diagonal terms $n = m$.

As a next step, we can carry out the summation over the discrete time $j$ in Eq. (13). Note that for all modes that satisfy $\varepsilon_n \neq 0, \pi$ we have $|\lambda_{n,\pm}| < 1$, showing that these modes all leave the system eventually. For these, the sum over $j$ is convergent and results in

$$\sum_{j\in\mathbb{Z}^+} |\Lambda_n(j)|^2 = 1. \tag{16}$$

Substituting this into Eq. (13) we obtain

$$\langle\langle \Delta x\rangle\rangle = \frac{2}{NL}\sum_n\left[\sum_{y,b} y\langle n|y,b\rangle\langle y,b|n\rangle - \sum_{x,a} x\langle n|x,a\rangle\langle x,a|n\rangle\right]. \tag{17}$$

Note that in the two terms above $x$ and $y$ play the same role. Therefore, we can bring the two terms into one sum to get the following formula for the double averaged displacement:

$$\langle\langle \Delta x\rangle\rangle = \frac{2}{LN}\sum_x x \sum_n \left[\sum_{b=N+1}^{2N} |\langle x,b|n\rangle|^2 - \sum_{a=1}^{N} |\langle x,a|n\rangle|^2\right]. \tag{18}$$

This has the interpretation of the combined sublattice polarization of all negative energy bands, since the index $n$ labels the states with $\varepsilon_n \leq 0$. We can make this result more compact by using the projector $\hat{Q}_-$ introduced in the main text. Then the average displacement becomes

$$\langle\langle \Delta x\rangle\rangle = \frac{2}{LN}\sum_x x \left[\sum_{b=N+1}^{2N} \langle x,b|\hat{Q}_-|x,b\rangle - \sum_{a=1}^{N} \langle x,a|\hat{Q}_-|x,a\rangle\right], \tag{19}$$

which is equivalent to the result stated in the main text:

$$\langle\langle \Delta x\rangle\rangle = \frac{2}{LN}\mathrm{Tr}\left\{\hat{X}\hat{\Gamma}\hat{Q}_-\right\}. \tag{20}$$

To see the validity of this formula, note that

$$\hat{\Gamma} = \hat{P}_A - \hat{P}_B = \sum_{x=1}^{L}\left[\sum_{a=1}^{N} |x,a\rangle\langle x,a| - \sum_{b=N+1}^{2N} |x,b\rangle\langle x,b|\right]. \tag{21}$$

Substituting this into Eq. (20) reduces it to Eq. (19).

The result for the double averaged dwell time $\langle\langle t\rangle\rangle$ can be derived in a similar manner. Using its definition and Eq. (12), $\langle\langle t\rangle\rangle$ is given by

$$\langle\langle t\rangle\rangle = \frac{4T}{NL}\sum_{n,m}\sum_{x,a}\langle n|x,a\rangle\langle x,a|m\rangle \sum_{y,b}\langle x,b|n\rangle\langle m|x,b\rangle \sum_j j\Lambda_n(j)\Lambda_m(j)^*. \tag{22}$$

Using the formulas (14) this reduces to

$$\langle\langle t\rangle\rangle = \frac{T}{NL}\sum_n\sum_j j\,|\Lambda_n(j)|^2 \tag{23}$$

We can once again perform the sum over $j$, provided that $\varepsilon_n \neq 0, \pi$, which yields

$$\sum_j j\,|\Lambda_n(j)|^2 = \frac{p_M}{(1+\sqrt{1-p_M})^2}\frac{1}{\sin^2\varepsilon_n} + \frac{2\sqrt{1-p_M}}{p_M}. \tag{24}$$

In the thermodynamic limit we can replace the sum over $n$ with an integral over the quasienergy $\varepsilon$ and recover the result of the main text. We note that it is possible to calculate analytically the variance $\langle\langle t^2\rangle\rangle - \langle\langle t\rangle\rangle^2$ along the same lines, i.e. by computing the sum $\sum_j j^2\,|\Lambda_n(j)|^2$.

## III. PROOF OF $\langle\langle \Delta x\rangle\rangle = \nu/N$

We now show that the formula (20) coincides with the real-space winding number defined by Mondragon-Shem et. al.

Writing out the commutator and using the cyclic periodicity of the trace we can write the winding number as

$$\nu = \frac{1}{L}\mathrm{Tr}\left\{\left(\hat{P}_A\hat{Q}\hat{P}_B^2\hat{Q}\hat{P}_A - \hat{P}_B\hat{Q}\hat{P}_A^2\hat{Q}\hat{P}_B\right)\hat{X}\right\}. \tag{25}$$

Using the definition $\hat{Q} = \hat{\Gamma}\hat{Q}_-\hat{\Gamma} - \hat{Q}_-$ we have the relations

$$\hat{P}_A\hat{Q}\hat{P}_B = -2\hat{P}_A\hat{Q}_-\hat{P}_B \qquad \hat{P}_B\hat{Q}\hat{P}_A = -2\hat{P}_B\hat{Q}_-\hat{P}_A, \tag{26}$$

and the winding number therefore becomes

$$\nu = \frac{4}{L}\mathrm{Tr}\ \left\{\left(\hat{P}_A\hat{Q}_-\hat{P}_B^2\hat{Q}_-\hat{P}_A - \hat{P}_B\hat{Q}_-\hat{P}_A^2\hat{Q}_-\hat{P}_B\right)\hat{X}\right\}. \tag{27}$$

At this point it is useful to introduce block matrices for the operators $\hat{Q}_-$ and $\hat{X}$ as

$$\hat{Q}_- = \begin{pmatrix}\mathbf{Q}_{AA} & \mathbf{Q}_{AB}\\ \mathbf{Q}_{BA} & \mathbf{Q}_{BB}\end{pmatrix} \qquad \hat{X} = \begin{pmatrix}\mathbf{X}_{AA} & \mathbf{X}_{AB}\\ \mathbf{X}_{BA} & \mathbf{X}_{BB}\end{pmatrix}, \tag{28}$$

where $\mathbf{Q}_{AA}$, includes all the matrix elements of $\hat{Q}_-$ between states of sublattice $A$, and similarly for the other blocks. The blocks obey $\mathbf{Q}_{AB} = \mathbf{Q}_{BA}^\dagger$ and $\mathbf{X}_{AB} = \mathbf{X}_{BA}^\dagger$ due to hermiticity.

Using these blocks we can write

$$\hat{P}_A\hat{Q}_-\hat{P}_B^2\hat{Q}_-\hat{P}_A - \hat{P}_B\hat{Q}_-\hat{P}_A^2\hat{Q}_-\hat{P}_B = \begin{pmatrix}\mathbf{Q}_{AB}\mathbf{Q}_{BA} & 0\\ 0 & -\mathbf{Q}_{BA}\mathbf{Q}_{AB}\end{pmatrix}, \tag{29}$$

so that the winding number becomes

$$\nu = \frac{4}{L}\mathrm{Tr}\ \{\mathbf{Q}_{AB}\mathbf{Q}_{BA}\mathbf{X}_{AA}\} - \frac{4}{L}\mathrm{Tr}\ \{\mathbf{Q}_{BA}\mathbf{Q}_{AB}\mathbf{X}_{BB}\}. \tag{30}$$

To proceed further we need the following two properties of $\hat{Q}_-$:

$$\hat{Q}_-^2 = \hat{Q}_- \qquad \hat{Q}_-\hat{Q}_+- = \hat{Q}_-\hat{\Gamma}\hat{Q}_-\hat{\Gamma} = 0. \tag{31}$$

The first of these translates for the blocks as

$$\mathbf{Q}_{AB}\mathbf{Q}_{BA} = \mathbf{Q}_{AA} - \mathbf{Q}_{AA}^2 \qquad \mathbf{Q}_{BA}\mathbf{Q}_{AB} = \mathbf{Q}_{BB} - \mathbf{Q}_{BB}^2 \tag{32}$$

and the second as

$$\mathbf{Q}_{AB}\mathbf{Q}_{BA} = \mathbf{Q}_{AA}^2 \qquad \mathbf{Q}_{BA}\mathbf{Q}_{AB} = \mathbf{Q}_{BB}^2. \tag{33}$$

From these it follows that

$$\mathbf{Q}_{AA}^2 = \mathbf{Q}_{AA}/2 \qquad \mathbf{Q}_{BB}^2 = \mathbf{Q}_{BB}/2. \tag{34}$$

Plugging these into Eq. (30) we arrive at

$$\nu = \frac{2}{L}\mathrm{Tr}\ \{\mathbf{Q}_{AA}\mathbf{X}_{AA}\} - \frac{2}{L}\mathrm{Tr}\ \{\mathbf{Q}_{BB}\mathbf{X}_{BB}\}. \tag{35}$$

Now let us turn our attention to the double averaged displacement. Using the block notation, Eq. (20) becomes

$$\langle\langle\Delta x\rangle\rangle = \frac{2}{NL}\left(\mathrm{Tr}\ \{\mathbf{Q}_{AA}\mathbf{X}_{AA}\} + \mathrm{Tr}\ \{\mathbf{Q}_{AB}\mathbf{X}_{BA}\} - \mathrm{Tr}\ \{\mathbf{Q}_{BA}\mathbf{X}_{AB}\} - \mathrm{Tr}\ \{\mathbf{Q}_{BB}\mathbf{X}_{BB}\}\right). \tag{36}$$

The second and third terms cancel each other since

$$\mathrm{Tr}\ \{\mathbf{Q}_{AB}\mathbf{X}_{BA}\} = [\mathrm{Tr}\ \{\mathbf{X}_{AB}\mathbf{Q}_{BA}\}]^* = \mathrm{Tr}\ \{\mathbf{X}_{AB}\mathbf{Q}_{BA}\}, \tag{37}$$

where in both equalities we used the fact that both $\hat{Q}_-$ and $\hat{X}$ are hermitian. Therefore, we are left with

$$\langle\langle\Delta x\rangle\rangle = \frac{2}{NL}\mathrm{Tr}\ \{\mathbf{Q}_{AA}\mathbf{X}_{AA}\} - \frac{2}{NL}\mathrm{Tr}\ \{\mathbf{Q}_{BB}\mathbf{X}_{BB}\}. \tag{38}$$

Comparison with Eq. (35) gives us the desired result:

$$\langle\langle\Delta x\rangle\rangle = \frac{\nu}{N}. \tag{39}$$
